# Supplementary material for: Can Mamba Learn How to Learn? A Comparative Study on In-Context Learning Tasks
Source: arXiv:2402.04248 source file (2024-04-25)
Supplement: Supplementary file 1 [file extended_related.tex]

\section{Extended Related Work}

We have two kinds of work to cover in detail:
Subquadratic architecture, Transformer ICL.
